# Supplementary material for: GMAI-VL & GMAI-VL-5.5M: A Large Vision-Language Model and A Comprehensive Multimodal Dataset Towards General Medical AI
Source: arXiv:2411.14522 source file (2025-03-27)
Supplement: Supplementary file 1 [file 6_suppl_bak.tex]

\clearpage
\setcounter{page}{1}
\maketitlesupplementary


\section{Training details with LLaVA-Med}
The training differences detailed in Table~\ref{table:training-strategy}.
\begin{table}[htpb]
\centering
\vspace{-3mm}
\caption{Training Strategy for Different Models}
\vspace{-3mm}
\setlength\tabcolsep{1pt}
\resizebox{0.95\linewidth}{!}{
\begin{tabular}{|c|c|c|c|c|c|c|}
\hline
\textbf{Training Method} & \multicolumn{2}{c|}{\textbf{Stage-1}} & \multicolumn{2}{c|}{\textbf{Stage-2}} & \multicolumn{2}{c|}{\textbf{Stage-3}} \\
\hline
\textbf{Model} & \textbf{Data} & \textbf{Training Module} & \textbf{Data} & \textbf{Training Module} & \textbf{Data} & \textbf{Training Module} \\
\hline
llava-med & only caption & projector & - & - & VQA & llm \& projector \\
\hline
qilin-vl-med & only caption & projector & - & - & VQA & llm \& projector \\
\hline
gmai-vl & VQA & projector & VQA & VE \& projector & VQA & fully finetune \\
\hline
\end{tabular}}
\vspace{-2mm}
\label{table:training-strategy}
\end{table}

\section{Benchmarks}
\label{sec:benchmarks}

To evaluate our model, we employed several established multimodal medical benchmarks, each targeting specific aspects of medical image understanding and question answering. Below is a brief overview of the benchmarks used in our experiments:

\begin{itemize}[leftmargin=*]
    \item \textbf{Traditional medical VQA benchmarks}:  
    % The traditional multimodal medical question-answering benchmarks, including PMCVQA~\citep{zhang2023pmc}, PathVQA~\citep{he2020pathvqa}, VQA-RAD~\citep{lau2018dataset}, and SLAKE~\citep{liu2021slake}, cover a variety of imaging modalities and textual tasks, primarily evaluating the model's ability to extract information from medical images and answer related clinical questions. They evaluate the model’s performance in understanding different medical imaging modalities and multimodal information integration.
    Traditional multimodal medical question-answering benchmarks, such as VQA-RAD~\citep{lau2018dataset}, SLAKE~\citep{liu2021slake}, and PMCVQA~\citep{zhang2023pmc}, span various imaging modalities tasks, primarily assessing the model’s ability to extract information from medical images and answer clinical questions. They evaluate the model’s performance in understanding medical imaging and integrating multimodal information.

    \vspace{1mm}
    \item \textbf{OmniMedVQA}:  
    OmniMedVQA~\citep{hu2024omnimedvqa} provides a rich dataset of paired medical images and text, designed to evaluate the model’s ability to recognize and understand fundamental medical imaging concepts, focusing on cross-modal reasoning and information integration.

    \vspace{1mm}
    \item \textbf{GMAI-MMBench}:  
    GMAI-MMBench~\citep{chen2024gmai} focuses on assessing the model’s ability to identify fine-grained objects in complex clinical scenarios, challenging its capacity to handle long-context tasks and accurately recognize and reason over detailed medical features.

    \vspace{1mm}
    \item \textbf{MMMU Health \& Medicine track}: 
    The Health \& Medicine track of the MMMU~\citep{yue2024mmmu} benchmark spans a wide range of medical fields, derived from university exams, quizzes, and textbooks. It evaluates the model’s reasoning ability in complex medical scenarios and the specialized knowledge in health and medicine.
\end{itemize}



\section{Expanded Data Generation Example}

In this section, we present the full version of Fig.~\ref{fig:prompt}, which provides a detailed example of the data generation process, as shown in Fig.\ref{fig:prompt_compare_large}. This expanded illustration includes the complete prompt and the corresponding detailed responses, enabling a clear comparison between data generation methodologies with and without annotation guidance. The detailed comparison allows for a more intuitive understanding of the distinctions between both methods.

\begin{figure*}[htbp]
    \centering
    \includegraphics[width=0.9\linewidth]{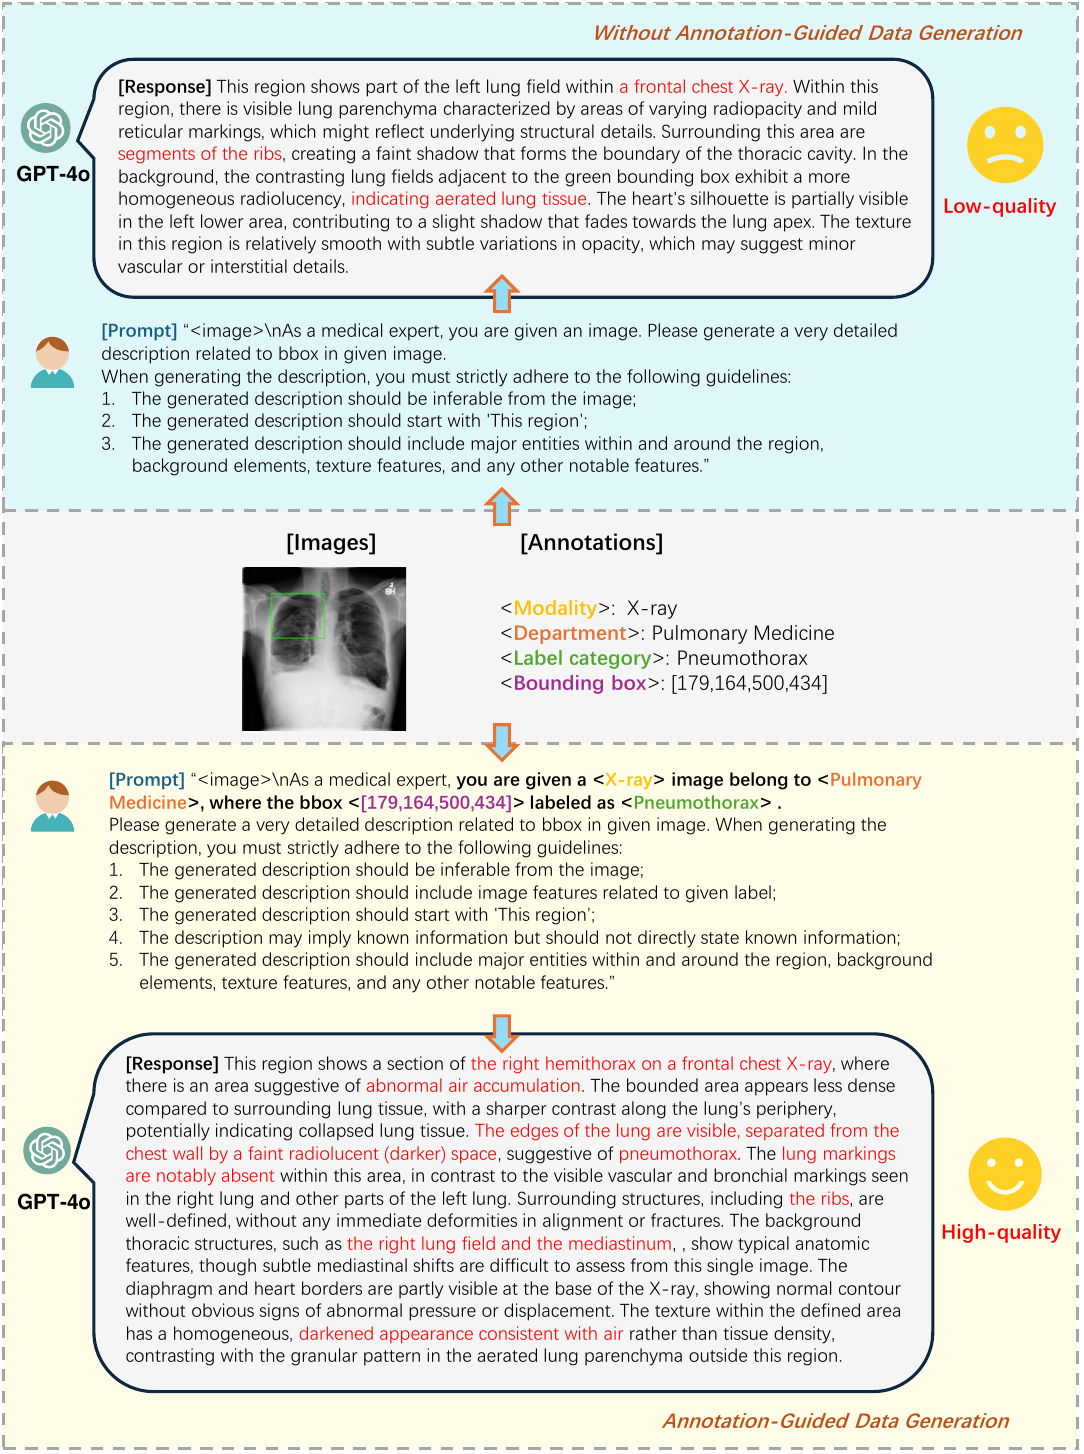}
    \caption{The full version of Fig.~\ref{fig:prompt} in the main text illustrates the complete of data generation pipeline， comparing without-annotation-guided and annotation-guided methods. The annotation-guided approach integrates specific annotation information (\textit{e.g.}, \texttt{<image, modality, label, department, bbox [optional]>}) to generate high-quality, accurate descriptions, while the without-annotation-guided approach often results in lower-quality outputs.}
    \label{fig:prompt_compare_large}
\end{figure*}


% \section{Data Filter}
% \label{sec:filter}
% Five PhD co-authors and two radiologists to manually review 100 samples from each dataset to verify data quality. Bad image quality, brief answers, and incorrect or irrelevant responses in image-text pairs are classified as low quality. Reviews are rated on a scale of 1 to 5. The final rating is determined by the weighted average score: PhDs weigh 1, radiologists weigh 2, and datasets with a weighted average score below 3 are classified as low quality.



\section{Details of GMAI-VL-5.5M}


\definecolor{blueColor}{HTML}{0054D6}

In Table.~\ref{tab:sub_dataset}, we provide sub-datasets information of the multimodal dataset GMAI-VL-5.5M we have constructed. Based on the different data forms introduced in the paper, we have categorized the data into five distinct sub-datasets. These include GMAI-MM-Caption-1.7M, GMAI-MM-Instruct-0.9M, GMAI-MM-Percept-1.3M, GMAI-Text-Single-1M, and GMAI-Text-0.6M. Each sub-dataset corresponds to specific components: image caption data, free instruction data, visual perception data, text-only, and conversation. Furthermore, Fig. \ref{fig:distributions} presents a comprehensive distribution of the data across different modalities, original tasks, departments, and clinical task within this multimodal dataset, highlighting its extensive richness and diversity.
% The data will be open-sourced in the above sections.
\input{tables/sub-dataset_details_of_GMAI-VL-MM-5.5M}

\section{Training Data Overview}
In this section, we provide a comprehensive overview of all datasets utilized for training the GMAI-VL model. The details include the dataset names, their corresponding categories, the amount of data used for training, and the proportion of training data allocated to each dataset during the three phases of model training.  Fig. \ref{fig:distribution_of_our_data} visualizes the distribution of all our training data, showing the proportion of each category and subcategory. 

Table.~\ref{tab:traing_dataset_list} summarizes the datasets employed, highlighting their respective categories and sizes. It is important to note that for certain datasets, we performed data cleaning and bilingual translation. As a result, the dataset sizes reported here may differ from the official numbers.

% the distribution of GMAI-VL-5.5M
% \begin{figure*}[!htbp]
%     \centering
%     % \includegraphics[width=\linewidth]{sources/figures/distribution_of_our_data.pdf}
%     \begin{minipage}{0.49\linewidth}
%         \centering
%         \includegraphics[width=0.95\linewidth]{figs/modality_of_our_data.pdf}
%         \subcaption*{\small(a) Modality distribution}
%     \end{minipage}
%     \hfill
%     \begin{minipage}{0.49\linewidth}
%         \centering
%         \includegraphics[width=0.89\linewidth]{figs/ori_task_of_our_data.pdf}
%         \subcaption*{\small(b) Original task distribution}
%     \end{minipage}
    
%     \vspace{0.1cm} % Add vertical space between rows

%     \begin{minipage}{0.49\linewidth}
%         \centering
%         \includegraphics[width=0.88\linewidth]{figs/department_of_our_data.pdf}
%         \subcaption*{\small(c) Department distribution}
%     \end{minipage}
%     \hfill
%     \begin{minipage}{0.49\linewidth}
%         \centering
%         \includegraphics[width=\linewidth]{figs/Clinical_task_of_our_data.pdf}
%         \subcaption*{\small(d) Clinical task distribution}
%     \end{minipage}
% \caption{
% %Distribution of GMAI-VL-15M across various modalities, departments, and tasks. 
% Distribution of GMAI-VL-5.5M across tasks, modalities, departments, and clinical tasks.  
% (a) Original Task Distribution: The dataset includes 2D Classification (50.4\%), 3D Segmentation (30.3\%), 2D Segmentation (12.7\%), and 2D Detection (6.6\%).  
% (b) Modality Distribution: In addition to CT (26.8\%) and MR (24.7\%), X-ray (12.6\%), Pathology (11.2\%), and less common modalities like Dermoscopy (3.5\%), Microscopy (2.4\%), and PET (0.2\%) are represented.  
% (c) Department Distribution: While Orthopedic Surgery (12.9\%) and General Surgery (10.3\%) are the top contributors, departments like Endocrinology (1.3\%), Infectious Diseases (0.8\%), and Urology (0.7\%) also provide data.  
% (d) Clinical Task Distribution: Besides Disease Diagnosis (40.4\%) and Organ Recognition (16.0\%), tasks such as Muscle Recognition (3.3\%), Nervous Tissue Recognition (1.5\%), and Microorganism Recognition (1.2\%) are included.
% Note: The distribution statistics shown here pertain only to the multimodal components of GMAI-VL-5.5M.
% }
% \label{fig:distributions}
% \end{figure*}


\begin{figure*}[htbp]
    \centering
    \includegraphics[width=1.0\linewidth]{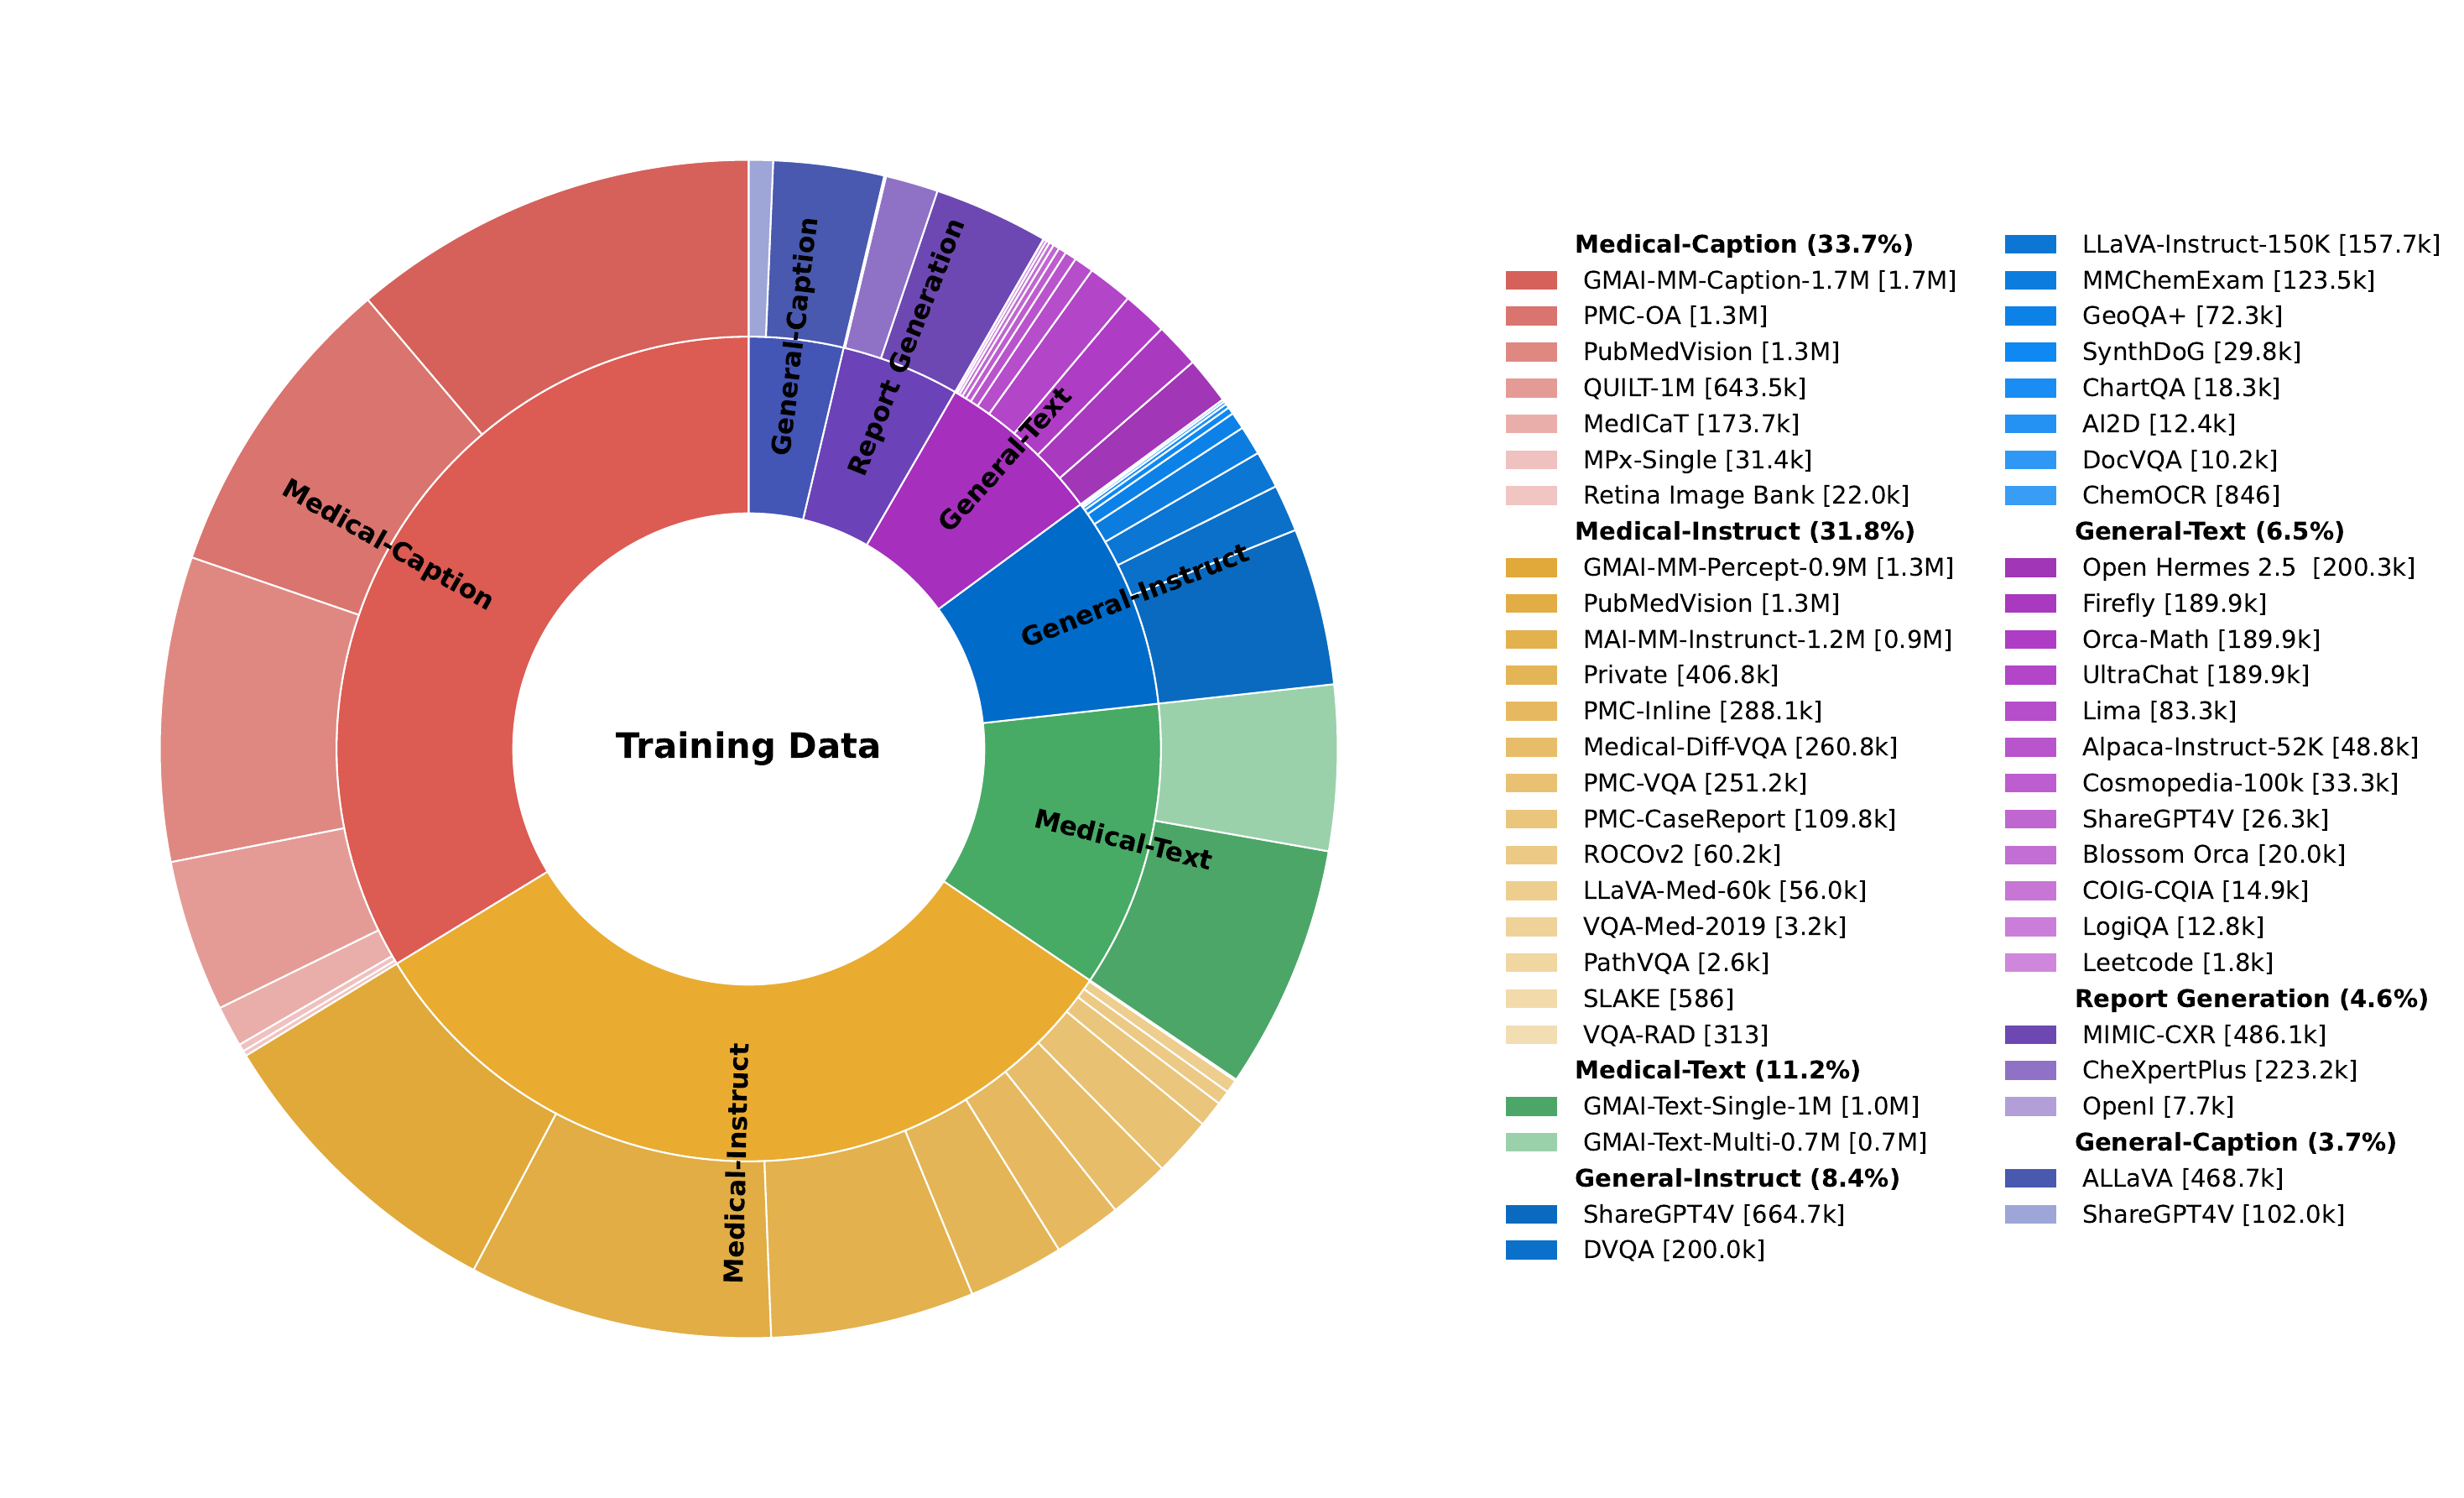}
    \caption{Distribution of all our training data. The inner ring represents major categories, each depicted in a different color. The outer ring corresponds to the subcategories within each major category. The size of each segment is proportional to the amount of data, as indicated in the legend, where the data volume for each subcategory is also provided.}
    \label{fig:distribution_of_our_data}
\end{figure*}

\input{tables/dataset_used_summary}
% The training data for our model is comprehensively categorized into various segments, reflecting a diverse range of sources. The primary categories include Medical Caption, General Caption, Medical Instruction, General Instruction, Medical Text, General Text, and Report Generation. Fig~\ref{fig:distribution_of_our_data} shows the distribution of these different types of data.

% Medical Caption (33.7\%)
% This category encompasses datasets such as GMAI-MM-Caption and PMC-OA, focusing on medical image captioning. It accounts for the largest portion of our training data, emphasizing the importance of medical-specific descriptions.

% Medical Instruction (31.8\%)
% Datasets like Med-Instruct and MultiMed-Instruct are included here, providing detailed instructions for medical tasks. This segment highlights the model's capacity to understand and execute medical-related instructions.

% Medical Text (11.2\%)
% This section includes datasets such as PubMed and PMC-Articles, offering a vast array of medical literature and documentation. It supports the model's text comprehension and generation capabilities in the medical domain.

% General Instruction (8.4\%)
% Datasets under this category, such as ShareGPT and DVQAv2, contribute to the model's ability to follow and generate general instructions beyond the medical scope.

% General Text (6.5\%)
% This includes datasets like Open Hermes and Orca-Math, which provide general knowledge and text generation capabilities, ensuring the model's versatility in non-medical contexts.

% Report Generation (4.6\%)
% Datasets such as MIMIC-CXR and CheXpertPlus are used for generating medical reports, a critical application in healthcare settings.

% General Caption (3.7\%)
% This category includes datasets like AI2D and ALLAVA, focusing on general image captioning, enhancing the model's ability to describe visual content.

% The distribution of these datasets is visually depicted in Figure 4, illustrating the comprehensive and balanced approach to training across various domains.

\begin{figure*}[htbp]
    \centering
    \includegraphics[width=0.8\linewidth]{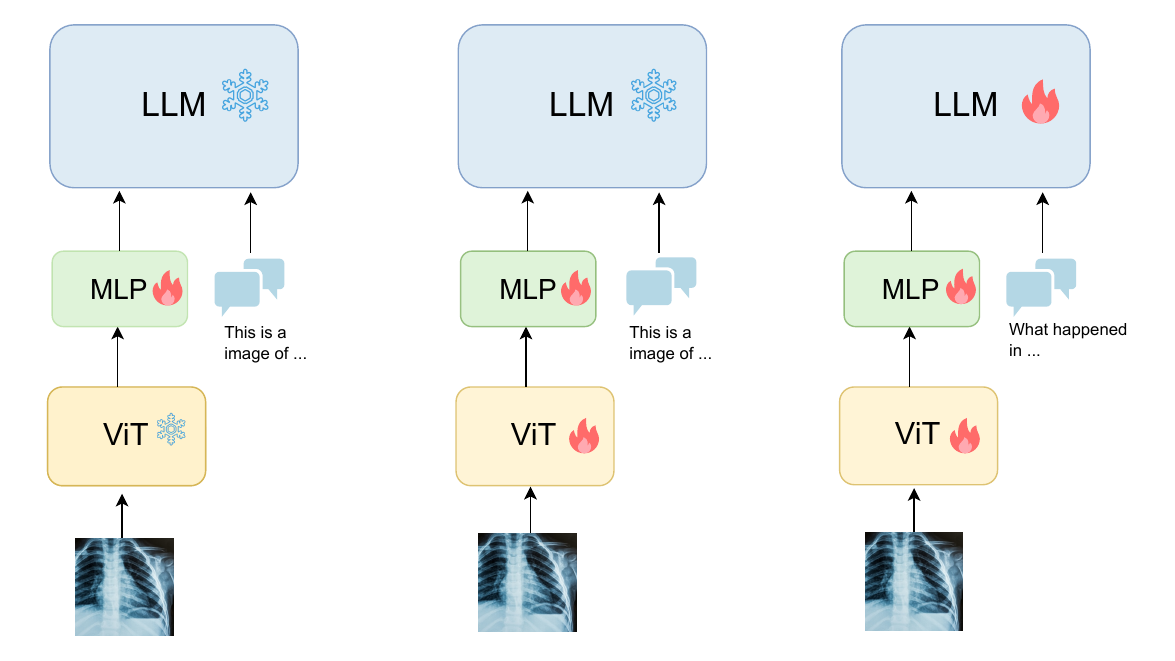}
    \caption{Diagram of the three-stage training process.}
    \label{fig:train_stage}
\end{figure*}

% \section{Model Training Settings}

% \input{tables/training_configuration}

% The table.~\ref{tab:setting} presents the training settings for GMAI-VL across three stages, detailing key hyperparameters. 
% The train diagram as illustrated in Fig.~\ref{fig:train_stage}.

% \begin{itemize}[leftmargin=*]
%     \item Stage I (Shallow alignment). 
%     During this stage, both the large language model (LLM) and the vision encoder are frozen, while the MLP remains trainable. The learning rate is set to \(1e^{-3}\) with a cosine decay schedule, using AdamW as the optimizer. Input size is \(336 \times 336\), and the total batch size is \(32 \times 8 \times 2\). Here, 32 refers to the number of GPUs used, 8 represents the micro-batch size per GPU, and 2 is the number of gradient accumulation steps. Notably, we use a soft packing technique, which allows each sample to actually contain multiple sequences—estimated at over 2 per sample. 
%     \item  Stage II (Deep alignment).
%     The LLM remains frozen, while the vision encoder and MLP are unfrozen and trainable, allowing for deeper feature alignment. The learning rate is lowered to \(1e^{-4}\), the total batch size is \(32 \times 4 \times 4\), and other settings remain consistent with Stage I.
%     \item Stage III (Instruction tuning).
%     In this stage, all components of the model are trainable, allowing for comprehensive fine-tuning. The learning rate is further reduced to \(1e^{-5}\), the total batch size is \(32 \times 4 \times 4\), while other parameters, including optimizer, remain unchanged across stages.    
% \end{itemize}
% Each stage utilizes DeepSpeed for mixed-precision training (bf16) on 32 A100 (80GB) GPUs. To accelerate the training rate of the model, we utilize the soft packing method in xtuner\footnote{https://github.com/InternLM/xtuner}, which packs multiple sequences into each sample to optimize memory usage and efficiency..


\section{GMAI-MMBench Results}
For further comparisons, Table~\ref{tab:gmai_full} provides additional results, including a broader range of models, such as Open-Source LVLMs, Proprietary LVLMs, and Medical Special Models.

\begin{table*}[t]
\centering
\caption{Results on the \textit{val} and \textit{test} sets of GMAI-MMBench for clinical VQA tasks. 
The full names of the evaluated tasks can be found in Table 5 in literature~\citep{chen2024gmai}. 
The best model in each category is in \textcolor{red}{red}, while the second-best is \textcolor{blue}{blue}.}
\resizebox{0.99\linewidth}{!}{
\setlength{\tabcolsep}{3.5pt}
\begin{tabular}{l|cc|cccccccccccccccccc}
\toprule
\multirow{2}{*}{\textbf{Model Name}}  
& \multirow{2}{*}{\makecell{\textbf{Overall}\\\textbf{(val)}}}
& \multirow{2}{*}{\makecell{\textbf{Overall}\\\textbf{(test)}}}
& \multirow{2}{*}{\textbf{AR}} & \multirow{2}{*}{\textbf{BVR}} & \multirow{2}{*}{\textbf{B}} 
& \multirow{2}{*}{\textbf{CR}} & \multirow{2}{*}{\textbf{C}}  & \multirow{2}{*}{\textbf{DD}} 
& \multirow{2}{*}{\textbf{IQG}}& \multirow{2}{*}{\textbf{MR}} & \multirow{2}{*}{\textbf{M}}  
& \multirow{2}{*}{\textbf{NT}} & \multirow{2}{*}{\textbf{OR-A}}& \multirow{2}{*}{\textbf{OR-HN}} 
& \multirow{2}{*}{\textbf{OR-P}}& \multirow{2}{*}{\textbf{OR-T}}& \multirow{2}{*}{\textbf{SG}}  
& \multirow{2}{*}{\textbf{SAR}}& \multirow{2}{*}{\textbf{SIR}}& \multirow{2}{*}{\textbf{SWR}}\\
\\
\midrule
\multicolumn{21}{c}{\cellcolor[HTML]{EFEFFF}\textbf{Random Guess}} \\
Random   & 25.70 & 25.94 & 38.20 & 22.73 & 22.92 & 22.72 & 24.06 & 26.66 & 27.13 
         & 27.00 & 20.00 & 24.75 & 21.37 & 22.93 & 22.33 & 21.18 & 32.43 & 24.23 
         & 21.39 & 23.71 \\
\midrule
\multicolumn{21}{c}{\cellcolor[HTML]{FFF3E4}\textbf{Open-Source LVLMs}} \\
Flamingo v2~\citep{awadalla2023openflamingo}
         & 25.58 & 26.34 & 37.74 & 21.50 & 20.62 & 22.00 & 22.41 & 27.29 & 25.91
         & 27.45 & 18.00 & 28.79 & 25.16 & 22.13 & 22.00 & 22.00 & 34.61 & 22.88
         & 20.44 & 27.43 \\
VisualGLM-6B~\citep{ding2021cogview}
         & 29.58 & 30.45 & 40.16 & 33.92 & 24.92 & 25.22 & 24.21 & 32.99 & 29.96
         & 29.53 & 21.20 & 37.88 & 30.32 & 24.80 & 13.33 & 29.88 & 33.11 & 19.62
         & 19.16 & 37.43 \\
InstructBLIP-7B~\citep{dai2024instructblip}
         & 31.80 & 30.95 & 42.12 & 26.92 & 24.92 & 28.09 & 21.65 & 34.58 & 31.58
         & 29.23 & 22.40 & 30.30 & 28.95 & 27.47 & 23.00 & 24.82 & 32.88 & 19.81
         & 21.64 & 26.57 \\
Qwen-VL~\citep{bai2023qwen}
         & 34.80 & 36.05 & 37.05 & 37.24 & 35.85 & 28.98 & 24.81 & 43.60 & 24.70
         & 30.12 & 19.20 & 44.44 & 29.68 & 31.87 & 25.00 & 31.18 & 30.26 & 21.54
         & 20.10 & 26.86 \\
Yi-VL-6B~\citep{young2024yi}
         & 34.82 & 34.31 & 41.66 & 39.16 & 26.62 & 30.23 & 31.88 & 38.01 & 26.72
         & 24.93 & 25.20 & 37.37 & 29.58 & 31.20 & 32.33 & 30.59 & 36.71 & 24.81
         & 23.18 & 31.43 \\
ShareGPT4V-7B~\citep{chen2023sharegpt4v}
         & 36.71 & 36.70 & 43.96 & 37.59 & 21.54 & 37.57 & 18.80 & 43.26 & 32.39
         & 27.30 & 22.80 & 43.43 & 29.47 & 37.33 & 22.00 & 31.76 & 34.98 & 24.42
         & 25.06 & 30.00 \\
LLAVA-V1.5-7B~\citep{liu2023llava}
         & 38.23 & 37.96 & 45.45 & 34.27 & 30.92 & 41.32 & 21.65 & 44.68 & 34.01
         & 27.74 & 23.60 & 43.43 & 28.00 & 42.13 & 29.00 & 35.06 & 33.41 & 22.12
         & 23.61 & 29.14 \\
XComposer2~\citep{internlmxcomposer2}
         & 38.68 & 39.20 & 41.89 & 37.59 & 33.69 & 40.79 & 22.26 & 45.87 & 36.44
         & 32.94 & 27.20 & 58.59 & 26.11 & 36.40 & 43.67 & 37.29 & 32.06 & 23.46
         & 27.80 & 32.86 \\
LLAVA-InternLM-7b~\citep{2023xtuner}
         & 38.71 & 39.11 & 36.36 & 36.54 & 32.62 & 38.10 & 30.68 & 46.53 & 34.82
         & 28.19 & 25.20 & 48.99 & 28.11 & 40.53 & 33.33 & 36.00 & 34.08 & 26.73
         & 24.12 & 29.71 \\
InternVL-Chat-V1.5~\citep{chen2024far}
         & 38.86 & 39.73 & 43.84 & 44.58 & 34.00 & 33.99 & 31.28 & 45.59 & 33.20
         & 38.28 & 32.40 & 42.42 & 31.89 & 42.80 & 27.00 & 36.82 & 34.76 & 23.27
         & 24.72 & 32.57 \\
InternVL-Chat-V1.2~\citep{chen2023internvl}
         & 39.52 & 40.01 & 41.66 & 44.06 & 27.38 & 38.46 & 34.29 & 46.99 & 33.60
         & 34.42 & 21.20 & 47.98 & 30.63 & 42.80 & 27.67 & 35.88 & 35.59 & \textcolor{blue}{23.85}
         & 24.98 & 28.00 \\
LLAVA-InternLM2-7b~\citep{2023xtuner}
         & 40.07 & 40.45 & 39.82 & 37.94 & 30.62 & 35.24 & 29.77 & 48.97 & 34.01
         & 25.96 & 20.80 & 53.03 & 30.95 & 42.67 & 32.00 & 39.88 & 32.43 & 21.73
         & 24.38 & 38.00 \\
DeepSeek-VL-7B~\citep{lu2024deepseek}
         & 41.73 & 43.43 & 38.43 & 47.03 & 42.31 & 37.03 & 26.47 & 51.11 & 33.20
         & 31.16 & 26.00 & 44.95 & 36.00 & 58.13 & 36.33 & 47.29 & 34.91 & 18.08
         & 25.49 & \textcolor{blue}{39.43} \\
MiniCPM-V2~\citep{xu2024llava-uhd}
         & 41.79 & 42.54 & 40.74 & 43.01 & 36.46 & 37.57 & 27.82 & 51.08 & 28.74
         & 29.08 & 26.80 & 47.47 & 37.05 & 46.40 & 25.33 & 46.59 & 35.89 & 22.31
         & 23.44 & 31.71 \\
\midrule
\multicolumn{21}{c}{\cellcolor[HTML]{FFF0F0}\textbf{Proprietary LVLMs}} \\
Claude3-Opus~\citep{anthropic2024claude}
         & 32.37 & 32.44 & 1.61  & 39.51 & 34.31 & 31.66 & 12.63 & 39.26 & 28.74
         & 30.86 & 22.40 & 37.37 & 25.79 & 41.07 & 29.33 & 33.18 & 31.31 & 21.35
         & 23.87 & 4.00 \\
Qwen-VL-Max~\citep{bai2023qwen}
         & 41.34 & 42.16 & 32.68 & 44.58 & 31.38 & 40.79 & 10.68 & 50.53 & 32.79
         & 44.36 & 29.20 & 51.52 & 41.37 & 58.00 & 30.67 & 41.65 & 26.95 & 25.00
         & 24.64 & 39.14 \\
GPT-4V~\citep{achiam2023gpt}
         & 42.50 & 44.08 & 29.92 & 48.95 & 44.00 & 37.39 & 12.93 & 52.88 & 32.79
         & 44.21 & \textcolor{blue}{32.80} & 63.64 & 39.89 & 54.13 & 37.00 & 50.59
         & 27.55 & 23.08 & 25.75 & 37.43 \\
Gemini 1.0~\citep{team2023gemini}
         & 44.38 & 44.93 & \textcolor{blue}{42.12} & 45.10 & 46.46 & 37.57 & 20.45
         & 53.29 & 35.22 & 36.94 & 25.20 & 51.01 & 34.74 & 59.60 & 34.00 & 50.00
         & \textcolor{blue}{36.64} & 23.65 & 23.87 & 35.43 \\
Gemini 1.5~\citep{reid2024gemini}
         & \textcolor{blue}{47.42} & \textcolor{blue}{48.36} & 43.50 & \textcolor{blue}{56.12}
         & \textcolor{blue}{51.23} & \textcolor{blue}{47.58} & 2.26  & \textcolor{blue}{55.33}
         & \textcolor{blue}{38.87} & \textcolor{blue}{48.07} & 30.00 & \textcolor{blue}{76.26}
         & \textcolor{blue}{51.05} & \textcolor{blue}{75.87} & 46.33 & 62.24 & 20.57 & 27.69
         & \textcolor{blue}{30.54} & 40.57 \\
GPT-4o~\citep{achiam2023gpt}
         & 53.53 & 53.96 & 38.32 & \textcolor{blue}{61.01} & \textcolor{blue}{57.08} 
         & \textcolor{blue}{49.02} & \textcolor{blue}{46.62} & 61.45 
         & \textcolor{red}{46.56} & 56.38 & 34.00 & 75.25 & 53.79 & 69.47 & 48.67
         & \textcolor{blue}{65.88} & 33.93 & 22.88 & 29.51 & 39.43 \\
\midrule
\multicolumn{21}{c}{\cellcolor[HTML]{EFEFEF}\textbf{Medical Special Model}} \\
Med-Flamingo~\citep{moor2023med}
         & 12.74 & 11.64 & 6.67  & 10.14 & 9.23  & 11.27 & 6.62  & 13.43 & 12.15
         & 6.38  & 8.00  & 18.18 & 9.26  & 18.27 & 11.00 & 11.53 & 12.16 & 5.19
         & 8.47  & 11.43 \\
LLaVA-Med~\citep{li2024llava}
         & 20.54 & 19.60 & 24.51 & 17.83 & 17.08 & 19.86 & 15.04 & 19.81 & 20.24
         & 21.51 & 13.20 & 15.15 & 20.42 & 23.73 & 17.67 & 19.65 & 21.70 & 19.81
         & 14.11 & 20.86 \\
Qilin-Med-VL-Chat~\citep{liu2023qilin}
         & 22.34 & 22.06 & 29.57 & 19.41 & 16.46 & 23.79 & 15.79 & 24.19 & 21.86
         & 16.62 & 7.20  & 13.64 & 24.00 & 14.67 & 12.67 & 15.53 & 26.13 & 24.42
         & 17.37 & 25.71 \\
RadFM~\citep{wu2023towards}
         & 22.95 & 22.93 & 27.16 & 20.63 & 13.23 & 19.14 & 20.45 & 24.51 & 23.48
         & 22.85 & 15.60 & 16.16 & 14.32 & 24.93 & 17.33 & 21.53 & 29.73 & 17.12
         & 19.59 & 31.14 \\
MedDr~\citep{he2024meddr}
         & 41.95 & 43.69 & 41.20 & 50.70 & 37.85 & 29.87 & 28.27 & 52.53 & 36.03
         & 31.45 & 29.60 & 47.47 & 33.37 & 51.33 & 32.67 & 44.47 & 35.14 & 25.19
         & 25.58 & 32.29 \\
\midrule
\multicolumn{21}{c}{\cellcolor[HTML]{EFFFFF}\textbf{Our Model}} \\
\textbf{GMAI-VL(w/o our data)}
         & \textcolor{blue}{54.99} & \textcolor{blue}{56.23} & \textcolor{blue}{51.26} 
         & \textcolor{red}{61.05} & 53.79 & 44.39 & 44.51 & \textcolor{blue}{62.60} 
         & 40.80 & \textcolor{blue}{57.42} & \textcolor{blue}{35.20} 
         & \textcolor{red}{79.50} & \textcolor{red}{61.31} & \textcolor{red}{77.81} 
         & \textcolor{red}{53.60} & \textcolor{red}{69.29} & 35.39 & \textcolor{blue}{35.77} 
         & 29.71 & \textcolor{blue}{44.86} \\

\textbf{GMAI-VL(ours)}
         & \textcolor{red}{61.74} & \textcolor{red}{62.43} & \textcolor{red}{75.26} 
         & 59.66 & \textcolor{red}{67.24} & \textcolor{red}{56.86} & \textcolor{red}{54.29} 
         & \textcolor{red}{67.14} & \textcolor{blue}{42.80} & \textcolor{red}{79.97} 
         & \textcolor{red}{41.60} & 75.00 & \textcolor{blue}{60.45} & 75.48 
         & \textcolor{blue}{53.33} & 58.12 & \textcolor{red}{42.09} & \textcolor{red}{72.31} 
         & \textcolor{red}{37.40} & \textcolor{red}{59.14} \\

\bottomrule
\end{tabular}
}
\label{tab:gmai_full}
\end{table*}


\section{Model Output Visualizations and Failure Case Studies}
\label{sec:case_vis}
\subsection{Model Output Visualization}
% Fig.~\ref{fig:vis_example} illustrates several examples of our model on various tasks including image description, disease diagnosis, diagnostic report generation, free question answering, etc. These examples cover a diverse range of medical imaging modalities and tasks, highlighting the model's versatility and general capabilities within medical domain. Furthermore, GMAI-VL supports both Chinese and English, thereby facilitating bilingual functionality and expanding its applicability in diverse clinical settings.
Fig.~\ref{fig:vis_example} presents several examples of model outputs on various tasks, including image description, disease diagnosis, diagnostic report generation, and free question answering. These examples span a wide range of medical imaging modalities and demonstrate the model's versatility and robustness across different tasks within the medical domain. Additionally, GMAI-VL supports both Chinese and English, which enhances its bilingual functionality and applicability in diverse clinical settings.

% \subsection{Failed Case Studies.} 
% From the bad case in Fig.~\ref{fig:bad}, it is evident that while GMAI-VL can diagnose diseases, it still struggles with subtle differences, such as severity (mild vs moderate).
% %We will provide detailed case studies in revised manuscripts, including both good cases and bad cases.
\subsection{Failure Case Studies}
Fig.~\ref{fig:bad} illustrates a failure case where GMAI-VL successfully identifies the presence of a disease but struggles with distinguishing between different severity levels (e.g., mild vs. moderate). This case highlights some of the current limitations of the model, particularly in scenarios involving subtle differences in medical conditions. Such cases emphasize the need for further refinement in the model's reasoning and decision-making capabilities, especially in complex diagnostic scenarios.

\begin{figure}[!ht]
    \centering
    \vspace{-3mm}
\includegraphics[width=\linewidth]{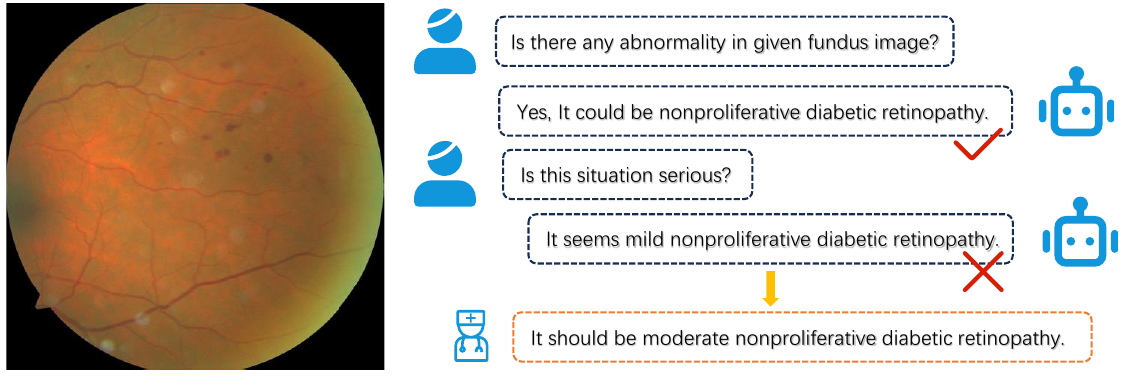}
    \vspace{-3mm}
    \caption{Bad case}
    \label{fig:bad}
    \vspace{-6mm}
\end{figure}


\begin{figure*}[p]
    \centering
    \includegraphics[width=\textwidth]{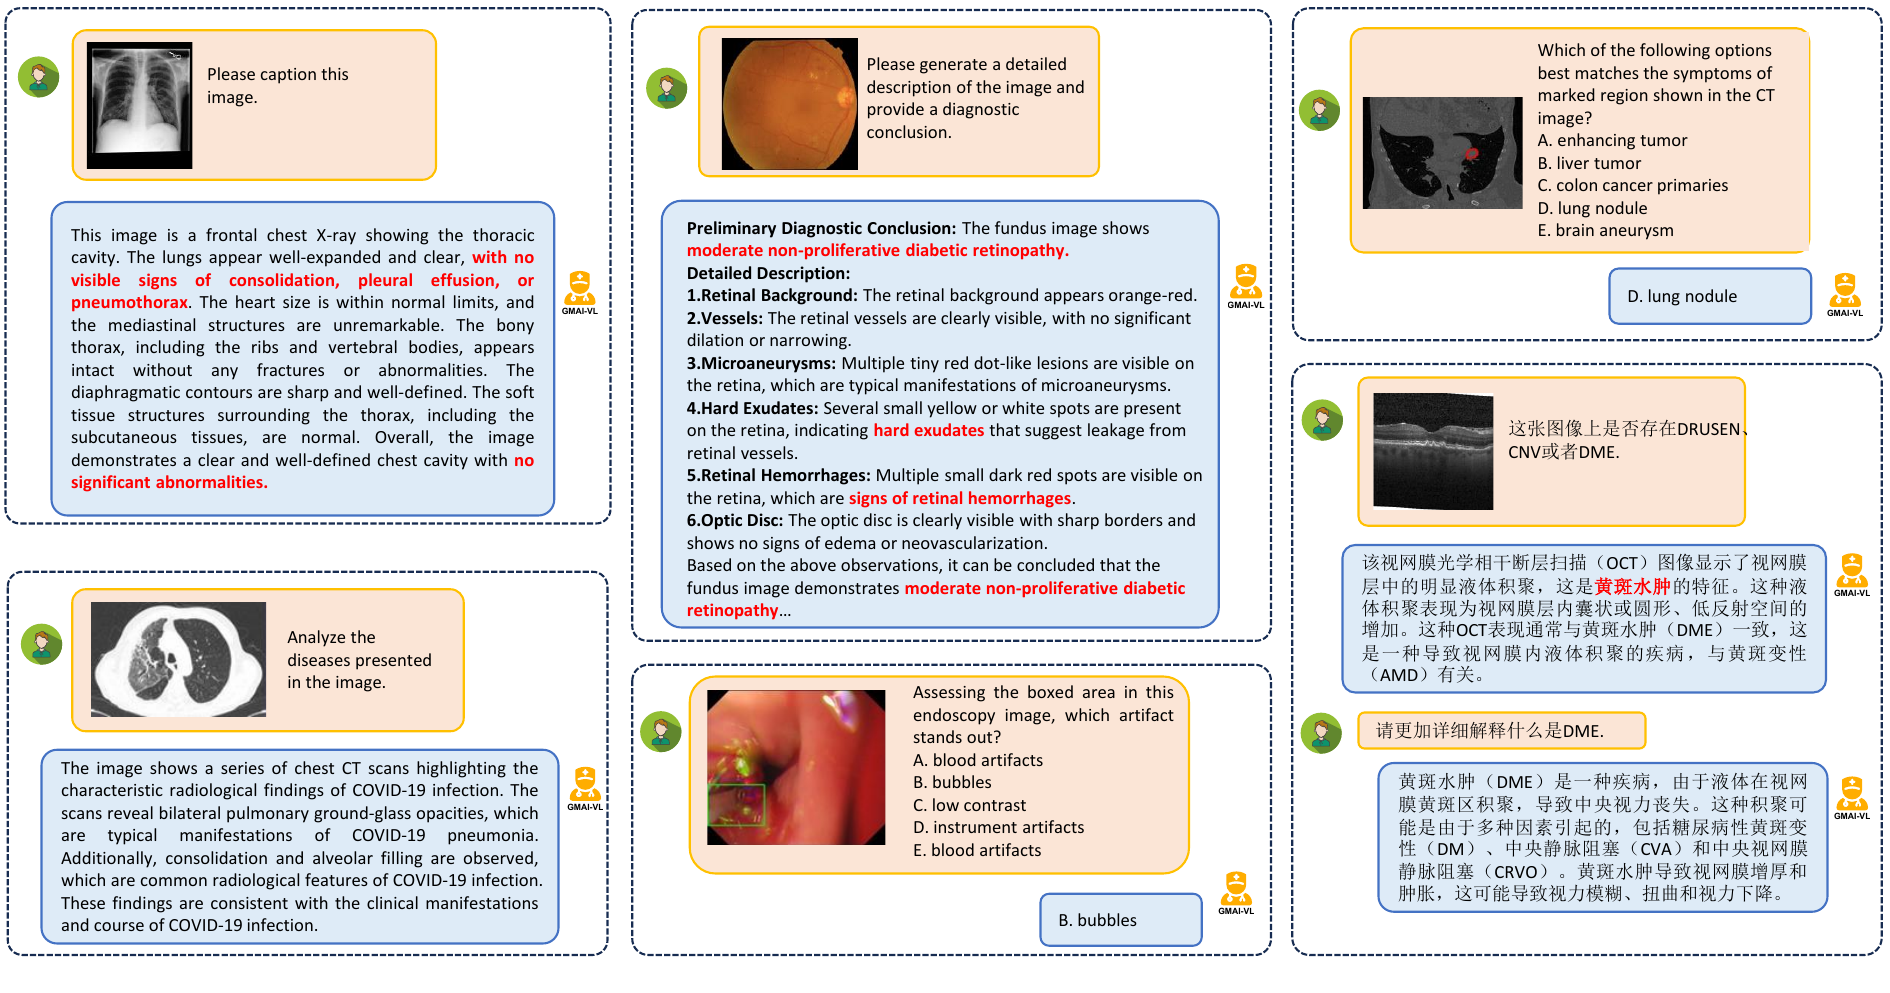}
    % \includegraphics[width=\linewidth]{figs/PIPELINE.drawio.svg}
    \caption{Examples of our model in various medical tasks, including image description, disease diagnosis, diagnostic report generation, free question answering, etc. The results demonstrate the model's versatility across different imaging modalities and tasks, with support for both Chinese and English.}
    \label{fig:vis_example}
    % \label{fig:distribution_of_our_data}
\end{figure*}





% \subsection{Curation Scope}


% \yf{Add your curation scope's explanation like below} 


% \paragraph{Microscopy} This category involves assessing the ability to generate microscopy descriptions of pathology images, focusing on clinically relevant features:

% \begin{itemize}[leftmargin=1em]
%     \item{Tissue Architecture and Arrangement}: Questions in this category should evaluate the understanding of overall tissue structure and spatial organization within a histological section. 
    
%     \item{Cytomorphological Characteristics}: These questions should focus on the detailed description of individual cell morphology, including nuclear and cytoplasmic features.

%     \item {Tumor Characteristics}: Questions under this category should assess the ability to identify and describe features specific to tumors, such as tumor cell differentiation, invasion, and specific patterns associated with different types of tumors.
    
%     \item {Histopathological Changes}: This category should include questions that evaluate the recognition and description of pathological changes in tissue, such as necrosis, inflammation, fibrosis, and other alterations that indicate disease processes.
% \end{itemize}

% \paragraph{Diagnosis} This category tests the ability of models to suggest a reasonable diagnosis based on histological images and relevant clinical context:

% \begin{itemize}[leftmargin=1em]
%     \item Disease Detection: Questions in this category should evaluate the model's ability to identify the presence or absence of a disease based on histological features and clinical information.
    
%     \item Disease Classification: These questions should focus on distinguishing between different types or subtypes of diseases, assessing the model’s capability to classify conditions accurately based on morphological and histopathological criteria.
    
%     \item Grading: Questions under this category should assess the model’s ability to determine the grade of a disease, particularly tumors, based on the degree of differentiation and cellular atypia observed in histological images.
    
%     \item Staging: This category should include questions that evaluate the ability to assign a stage to a disease, particularly in oncology, by assessing the extent of disease spread and involvement of surrounding tissues or organs.
    
%     \item Differential Diagnosis: Questions should test the model’s ability to provide a differential diagnosis, distinguishing between multiple potential conditions that may present with similar histological and clinical features.
% \end{itemize}



% \paragraph{Clinical} This category tests the ability of models to retrieve and apply clinically relevant background knowledge about diseases:

% \begin{itemize}[leftmargin=1em]
%     \item Treatment Guidance: Questions in this category should assess the model's ability to recommend appropriate treatment options based on the disease in question, considering factors such as disease stage, patient demographics, and any specific clinical guidelines.
    
%     \item Prognostic Assessment: These questions should focus on evaluating the model's ability to predict the likely course and outcome of a disease, including survival rates, potential complications, and long-term outcomes based on clinical and pathological data.
    
%     \item Risk Factors: Questions under this category should test the model's knowledge of risk factors associated with specific diseases, including genetic, environmental, and lifestyle factors that may influence disease development or progression.
    
%     \item Biomarker Analysis: This category should include questions that evaluate the ability to identify and interpret biomarkers relevant to the diagnosis, prognosis, or treatment of diseases, emphasizing their role in personalized medicine and targeted therapy.
% \end{itemize}

% \subsection{Bechmark Comparsion}
% Add comparison between our benchmark as well as other , for example, WSI-Caption, WSI-VQA


% \begin{table}[h!]
%     \centering
%     \resizebox{0.99\textwidth}{!}{
%     \begin{tabular}{l}
%         \toprule
%         \textbf{classification prompt} \\ % Replacing \[classification prompt\] with normal text
%         \rowcolor{gray!10} % 给这一行添加浅灰色背景
%         <image> As a medical expert, you are given a \textless modality \textgreater image. Please generate a very detailed description related to in the given image. \\
%         \rowcolor{gray!10} % 给这一行添加浅灰色背景
%         When generating the description, you must strictly adhere to the following guidelines: \\
%         \rowcolor{gray!10} % 给这一行添加浅灰色背景
%         1. The generated description should be inferable from the image; \\
%         \rowcolor{gray!10} % 给这一行添加浅灰色背景
%         2. The generated description should start with 'This image'; \\
%         \rowcolor{gray!10} % 给这一行添加浅灰色背景
%         3. The generated description should include major entities within and around the image, background elements, texture features, and any other notable features. \\
%         \midrule
%         \textbf{detection prompt} \\ % Replacing \[detection prompt\] with normal text
%         \rowcolor{gray!10} % 给下一行添加较深的灰色背景
%         As a medical expert, you are given a \textless modality\textgreater image belong to \textless department\textgreater, where the \textless bbox [x,x,x,x]\textgreater labeled as \textless label\textgreater. \\
%         \rowcolor{gray!10} % 给这一行添加浅灰色背景
%         Please generate a very detailed description related to bbox in given image. When generating the description, you must strictly adhere to the following guidelines: \\
%         \rowcolor{gray!10} % 给这一行添加浅灰色背景
%         1. The generated description should be inferable from the image; \\
%         \rowcolor{gray!10} % 给这一行添加浅灰色背景
%         2. The generated description should include image features related to given label; \\
%         \rowcolor{gray!10} % 给这一行添加浅灰色背景
%         3. The generated description should start with 'This region'; \\
%         \rowcolor{gray!10} % 给这一行添加浅灰色背景
%         4. The description may imply known information but should not directly state known information; \\
%         \rowcolor{gray!10} % 给这一行添加浅灰色背景
%         5. The generated description should include major entities within and around the region, background elements, texture features, and any other notable features. \\
%         \bottomrule
%     \end{tabular}}
% \end{table}


% \begin{table*}[h!]
%     \centering
%     \begin{tabular}{|p{\textwidth}|}
%         \toprule
%         \multicolumn{1}{|c|}{\textbf{classification prompt}} \\
%         \midrule
%         \begin{minipage}{1.0\textwidth} % Upper part (classification prompt)
%             \begin{minipage}{0.3\textwidth} % Left: Image
%                 \centering
%                 \includegraphics[width=0.6\linewidth]{figs/cls_sample.png}  % Replace with your image file
%                 % \captionof{figure}{Example Image}  % Optional: Add a caption if needed
%             \end{minipage} 
%             \hfill
%             \begin{minipage}{0.65\textwidth} % Right: Text content
%                 As a medical expert, you are given a \textless modality \textgreater image. Please generate a very detailed description related to the given image. \\
%                 When generating the description, you must strictly adhere to the following guidelines: \\
%                 1. The generated description should be inferable from the image; \\
%                 2. The generated description should start with 'This image'; \\
%                 3. The generated description should include major entities within and around the image, background elements, texture features, and any other notable features. \\
%             \end{minipage}
%         \end{minipage} \\
%         \midrule
%         \textbf{Output:} This region shows a section of the right hemithorax on a frontal chest X-ray, where there is an area suggestive of abnormal air accumulation. The bounded area appears less dense compared to surrounding lung tissue, with a sharper contrast along the lung’s periphery, potentially indicating collapsed lung tissue. The edges of the lung are visible, separated from the chest wall by a faint radiolucent (darker) space, suggestive of pneumothorax. The lung markings are notably absent within this area, in contrast to the visible vascular and bronchial markings seen in the right lung and other parts of the left lung. Surrounding structures, including the ribs, are well-defined, without any immediate deformities in alignment or fractures. The background thoracic structures, such as the right lung field and the mediastinum, show typical anatomic features, though subtle mediastinal shifts are difficult to assess from this single image. The diaphragm and heart borders are partly visible at the base of the X-ray, showing normal contour without obvious signs of abnormal pressure or displacement. The texture within the defined area has a homogeneous, darkened appearance consistent with air rather than tissue density, contrasting with the granular pattern in the aerated lung parenchyma outside this region. \\
%         \midrule
%         \multicolumn{1}{|c|}{\textbf{detection prompt}} \\
%         \midrule
%         \begin{minipage}{1.0\textwidth} % Upper part (detection prompt)
%             \begin{minipage}{0.3\textwidth} % Left: Image
%                 \centering
%                 \includegraphics[width=\linewidth]{figs/det_sample.png}  % Replace with your image file
%                 % \captionof{figure}{Example Image}  % Optional: Add a caption if needed
%             \end{minipage} 
%             \hfill
%             \begin{minipage}{0.65\textwidth} % Right: Text content
%                 As a medical expert, you are given a \textless modality\textgreater image belonging to \textless department\textgreater, where the \textless bbox [x,x,x,x]\textgreater is labeled as \textless label\textgreater. \\
%                 Please generate a very detailed description related to bbox in the given image. When generating the description, you must strictly adhere to the following guidelines: \\
%                 1. The generated description should be inferable from the image; \\
%                 2. The generated description should include image features related to the given label; \\
%                 3. The generated description should start with 'This region'; \\
%                 4. The description may imply known information but should not directly state known information; \\
%                 5. The generated description should include major entities within and around the region, background elements, texture features, and any other notable features. \\
%             \end{minipage}
%         \end{minipage} \\
%         \midrule
%         \textbf{Output:} This region shows a section of the right hemithorax on a frontal chest X-ray, where there is an area suggestive of abnormal air accumulation. The bounded area appears less dense compared to surrounding lung tissue, with a sharper contrast along the lung’s periphery, potentially indicating collapsed lung tissue. The edges of the lung are visible, separated from the chest wall by a faint radiolucent (darker) space, suggestive of pneumothorax. The lung markings are notably absent within this area, in contrast to the visible vascular and bronchial markings seen in the right lung and other parts of the left lung. Surrounding structures, including the ribs, are well-defined, without any immediate deformities in alignment or fractures. The background thoracic structures, such as the right lung field and the mediastinum, show typical anatomic features, though subtle mediastinal shifts are difficult to assess from this single image. The diaphragm and heart borders are partly visible at the base of the X-ray, showing normal contour without obvious signs of abnormal pressure or displacement. The texture within the defined area has a homogeneous, darkened appearance consistent with air rather than tissue density, contrasting with the granular pattern in the aerated lung parenchyma outside this region. \\
%         \bottomrule
%     \end{tabular}
% \end{table*}
